# Supplementary material for: Temperature-pressure scaling for air-fluidized grains on approaches to Point J
Source: arXiv:1110.5611 source file (2011-10-25)
Supplement: Supplementary file 1 [file Supplement_PressureTilt.pdf]

# Supplemental material for "Temperature-pressure scaling for air-fluidized grains..."

L. J. Daniels[1], T. K. Haxton[2], N. Xu[3], A. J. Liu[1], and D. J. Durian[1]
[1] *Department of Physics and Astronomy, University of Pennsylvania, Philadelphia, PA 19104-6396, USA*
[2] *Molecular Foundry, Lawrence Berkeley National Laboratory, Berkeley, CA 94720, USA and*
[3] *Department of Physics, University of Science and Technology of China, Hefei, Anhui, 230026, P.R. China*

Here we supply further technical details about the experiments, the analysis procedures, and the simulations. We also give system information and additional plots for the earlier data included in the main text. And finally we investigate the growth of dynamical heterogeneities as a function of the same dimensionless relaxation time, $\tau(P\sigma^{d-2}/m)^{1/2}$, used in the main text.

## I. EXPERIMENTAL DETAILS

The fluidization apparatus consists of a rectangular windbox, $1.5 \times 1.5 \times 4$ ft$^3$, a blower attached to the base, and a circular brass testing sieve with mesh size 150 $\mu$m and radius 15.3 cm that rests horizontally on top [1–5]. An insert with a square opening, (14.9 cm)$^2$, is oriented such that two sides of the opening lie parallel to the tilt axis of the apparatus. If misaligned, or if the system is not level parallel to the tilt axis, then convection currents can arise. The airspeed is small compared to the terminal falling speed of the beads, but large enough that turbulence excites random motion such that the beads roll without slipping.

The beads are illuminated from above by six 100 W incandescent bulbs arranged in a 1 ft diameter ring positioned 3 ft above the sieve. A digital CCD camera placed at the center of this ring captures the raw video data, typically for 20 minutes at a time at 120 frames per second. Since light is specularly reflected from the the top of the steel beads into the camera, the beads appear primarily as small dots in the video data. The dots for the two sizes of beads are different enough in size that big and small beads are easily distinguished and tracked. Post-processing of the video data is accomplished using LabVIEW, using custom code. The resulting $\{x(t), y(t)\}$ trajectory data for each of the 796 beads is smoothed using a running average with Gaussian window, yielding estimates of the error in the position data of $\pm 20$ $\mu$m.

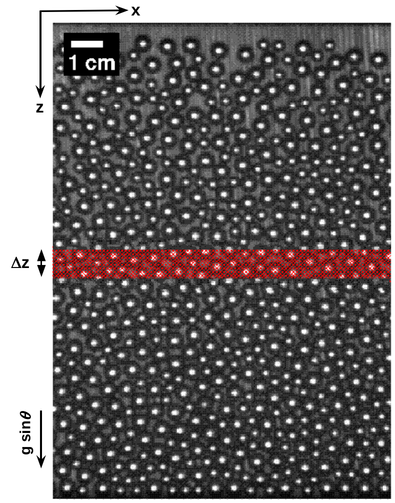


FIG. 1: (jamsystem.pdf) Raw video frame for a monolayer of bidisperse steel beads fluidized by an upflow of air. Here the tilt angle is $\theta = 0.72°$. The red horizontal bar with width $\Delta z = 0.84$ cm is an example of the typical strip size into which we divide the system in order to calculate depth-dependent quantities. We only show the region of the system for which we analyze data.

## II. DATA ANALYSIS

All quantities in the main text are deduced as a function of depth, $z$, down the slope of the sample plane, by splitting apart the trajectories into segments in which the particles remain within narrow strips, $\Delta z = 0.84$ cm. We discard any trajectory segment in which the bead passes within four diameters of the side walls. An example video frame, with one highlighted strip, is shown in Fig. 1. Note that the packing density increases with depth. The origin, $z = 0$, is taken in this plot to be at the top of the square sample area; this choice does not affect any of the analysis.

Example results for the mean-squared displacement (MSD), $\langle [x(t + \Delta t) - x(t)]^2 \rangle$, transverse to the $g \sin\theta$ in-plane component of gravity, are plotted vs delay time $\Delta t$ in Fig. 2 for both large and small beads at a range of depths. Each curve is time-averaged over all particle trace segments within the strip at the given depth. Note that the data in Fig. 2 show all of the characteristics associated with dynamics on approach to jamming: At the shortest delay times, the motion is ballistic, MSD $= \langle {v_x}^2 \rangle \Delta t^2$, and hence can be used to determine the beads' average kinetic energy, $(1/2)(m+I/r^2)\langle {v_x}^2 + {v_y}^2 \rangle$, which defines the effective temperature. Here $m$ and $I$ are the bead mass and moment of inertia, respectively. At the longest delay times, the motion is diffusive, MSD $\propto \Delta t$. At shallow depths the dynamics crosses over quickly from ballistic to diffusive, while at greater depths the dynamics develop an intermediate subdiffusive plateau that grows with depth on approach to jamming.

The relaxation times in the main text are deduced from when the MSD reaches $\sigma^2$, the square of the small particle diameter. For shallow depths this may be found directly from the data. For great enough depths, how-

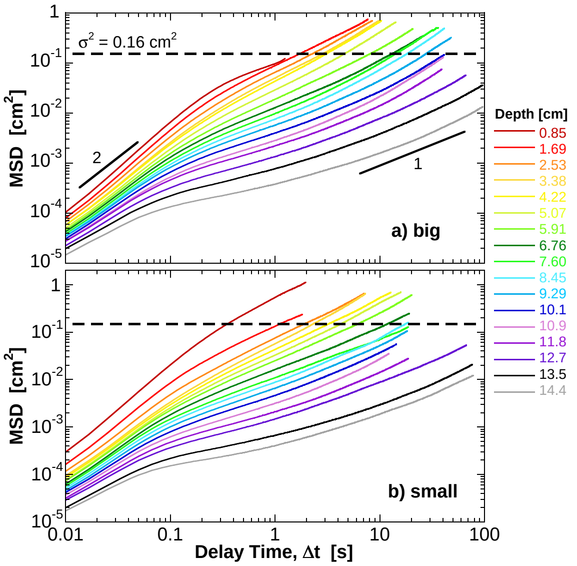


FIG. 2: (msd018.pdf) Mean-squared horizontal displacement vs delay time for a) big beads and b) small beads, at different depths as labeled. Here, the tilt angle is $\theta = 0.18°$. The dashed horizontal line in each plot is the squared small-bead diameter.

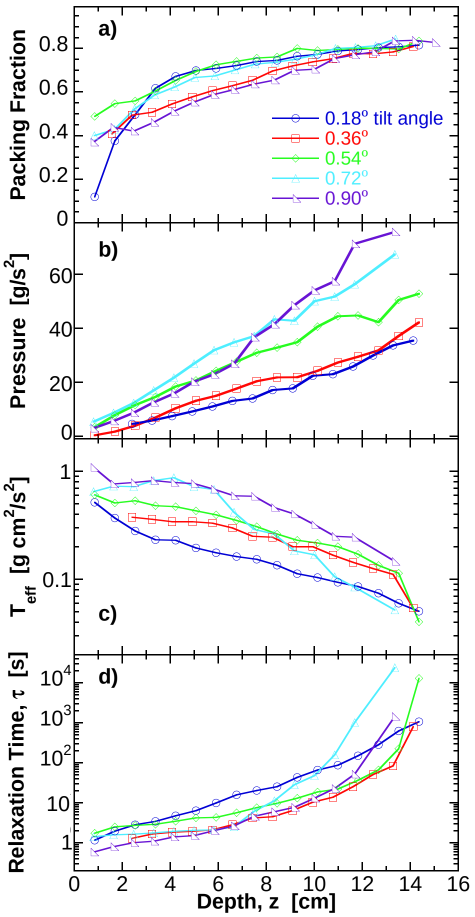


FIG. 3: (qsvz.pdf) a) Packing fraction, b) pressure, c) effective temperature, and d) relaxation time as a function of depth down the plane for a monolayer of air-fluidized beads tilted at different tilt angles as labeled.

ever, it is necessary to extrapolate using MSD $\propto \Delta t$. The various MSD curves end abruptly, at different delay times, according to minimum duration of the trajectories segments of all beads at the given depth. If the strip width, $\Delta z$, is increased, then the mean squared displacements can be measured to longer delay times; however, then there are fewer points and there will be significant variation of pressure, temperature, and packing fraction across the strip.

As an aside, we note that convection due to misalignment of the insert would show up in the MSD plot as superdiffusive dynamics at the longest times. This is clearly insignificant. We also verify that size segregation does not affect our data. However, the large beads have greater mass per unit area and hence can slowly work their way to the bottom of the sample while the small beads rise. To determine whether this size segregation is significant, we compute the quantity $N_{big}/(N_{big}+N_{small})$ as a function of depth down the plane, where $N_{big}$ is the number of large beads at that depth and $N_{small}$ the number of small beads. This quantity will equal 0.5 if a given region has equal numbers of each bead size, 0 if there are only small beads, and 1 if there are only large beads. We find that this quantity is very close to 0.5 at all depths for all systems that we have analyzed. However, for tilt angles larger than the maximum of 0.9° used here, segregation becomes noticeable for 20-30 minute duration runs.

For completeness, the entire final data set for packing fraction, pressure, temperature, and relaxation time are plotted vs depth $z$ in Fig. 3, for all five tilt angles. These same data are shown in the first figure of main text, plotted parametrically vs pressure.

## III. SIMULATION DETAILS

We conduct event-driven molecular dynamics simulations [6, 7] of 1024 two-dimensional hard disks in the microcanonical ensemble under periodic boundary conditions. As in the experiments, we study a binary mixture, half with diameter $\sigma$ and mass $m$ and half with diameter $1.4\sigma$ and mass $1.4^3 m$. The event-driven algorithm solves the Newtonian dynamics of perfectly hard disks that interact only via instantaneous, perfectly elastic collisions, and otherwise travel ballistically. Although the algorithm conserves energy, we periodically rescale the velocities to remove a small amount of numerical drift in the energies. Since there are no internal energy scales in the hard-sphere system, the only meaningful control parameters are the packing fraction $\phi$ or the dimensionless ratio $T/P\sigma^d$. The two are not independent; rather, they are related to each other by the equation of state.

Note also that the simulations are in the low $P\sigma^d/\epsilon$ limit, where $\epsilon$ is the interaction strength, since $\epsilon = \infty$ for hard spheres.

We conduct 76 simulations for packing fractions between 0.36 and 0.792. We initialize each simulation by slowly compressing the system from a previously equilibrated system at a lower packing fraction. We compress over a time interval equal to between $40\tau$ and $2000\tau$, where $\tau$ is the relaxation time. We then evolve the system for the same amount of time before conducting production runs lasting between $400\tau$ and $10000\tau$. During the production runs, we measure the pressure and the relaxation time, which we define as in the experiments as the time for the root mean-square-displacement to equal $\sigma$. We find that using such long simulations limits the scatter in the relaxation time and equation of state plots to be smaller than the width of the curves.

## IV. EARLIER DATA

Relaxation times were extracted from the MSD data of Refs. [2–5], and included in the scaling plot $\tau(P/m)^{1/2}$ vs $T/P\sigma^2$ of the main text. In Table I we collect the bead material and size information and contrast it with that for the present tilting experiments. In Fig. 4 we replot all relaxation time data, now vs packing fraction and also using symbols to distinguish the different earlier data sets.

| System | Material | $\sigma$ (cm) | $\sigma_{big}/\sigma$ | U (cm/s) |
|---|---|---|---|---|
| [2] PRE 2006 | steel | 0.635 | 1.38 | 950 |
| [3] PRE 2007 | steel | 0.318 | 1.25 | 545 |
| [4] Nat.Phys. 2007 | steel | 0.318 | 1.25 | 545 |
| [5] PRL 2008 | PP | 2.54 | 1.13 | 350−950 |
| Main text | steel | 0.397 | 1.40 | 700 |

TABLE I: Bead specifications for all experiments analyzed in the main text: diameter $\sigma$ of the smaller bead, large to small bead diameter ratio $\sigma_{big}/\sigma$, and superficial air speed $U$ given by volume flow rate per sample area. The density of the steel beads is 7.8 g/cm$^3$. The masses of the hollow polypropylene (PP) spheres are 3.0 g and 2.2 g. All systems are 1:1 bidisperse mixtures. The air speeds are always such that the beads roll without slipping.

## V. DYNAMICAL HETEROGENEITIES

The growth of the relaxation time is not caused by an obvious change in structure, in contrast to a growing static correlation length in ordinary second order phase transitions. However, there are growing length scales associated with dynamical effects such as the low frequency linear response and the spatiotemporally heterogenous nature of rearrangements [8–11]. For the latter, string-like swirls of mobile particles come and go in a back-

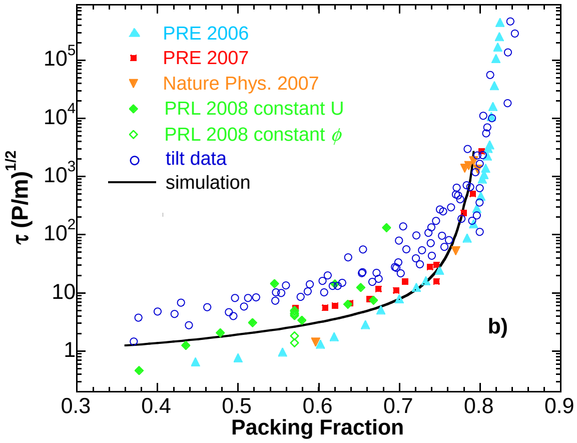


FIG. 4: (trelaxvphiB.pdf) Relaxation time $\tau$, made dimensionless by a factor of square root of pressure $P$ divided by small bead mass $m$, plotted versus packing fraction. Results are shown for both earlier data from Refs.[2–5], as well as for the tilt experiments and the thermal hard-sphere simulation of the main text, as labeled.

ground of less mobile particles. This may be characterized by the peak height $\chi_4{}^*$ of a four-point dynamical susceptibility [8], which in turn may be related to the average number $n^*$ of particles in the fast moving regions [3].

The growth of dynamical heterogeneities on approach to jamming has been measured previously for monolayers of air-fluidized beads, and reported as functions of experimental control parameters and effective temperature [3–5]. Here we consider the growth of $n^*$ as a function of the same dimensionless relaxation time $\tau(P/m)^{1/2}$ used in the main text. For the prior experiments [3–5], we deduce the dimensionless relaxation time using the known packing fraction and the scaling plot of $\tau(P/m)^{1/2}$ of the main text. For the new tilt experiments, at each strip of width $\Delta z$, we use the measured value of $\tau(P/m)^{1/2}$ and we compute $n^*$ from $\chi_4{}^*$ in terms of a video-based order parameter just as in Refs. [12, 13]. All results are collected in Fig. 5 as semilogarithmic and log-log plots of $\tau(P/m)^{1/2}$ vs $n^*$. First note that all data collapse, though there is considerable scatter. Even though the new tilt data are analyzed in thin strips, and even though the heterogeneities are extended objects, we find essentially the same $n^*$ results as in the prior experiments on uniform systems. Note, too, that the data nicely approach $\tau(P/m)^{1/2} = n^* = 1$ far from jamming. This, and the collapse, give further evidence for $\tau(P/m)^{1/2}$ as the correct dimensionless time scale.

The two sets of axes in Fig. 5 were chosen since most models predict that $n^*$ grows either logarithmically or as a power-law with relaxation time [9]. The former form is a straight line in Fig. 5a, which is not very unsatisfactory. A power law fit, $\tau(P/m)^{1/2} = (0.4 \pm 0.2)(n^*)^{2.9\pm0.8}$, is a straight line in Fig. 5b and gives a better description. The exponent is consistent with separate fits quoted in Ref. [5]

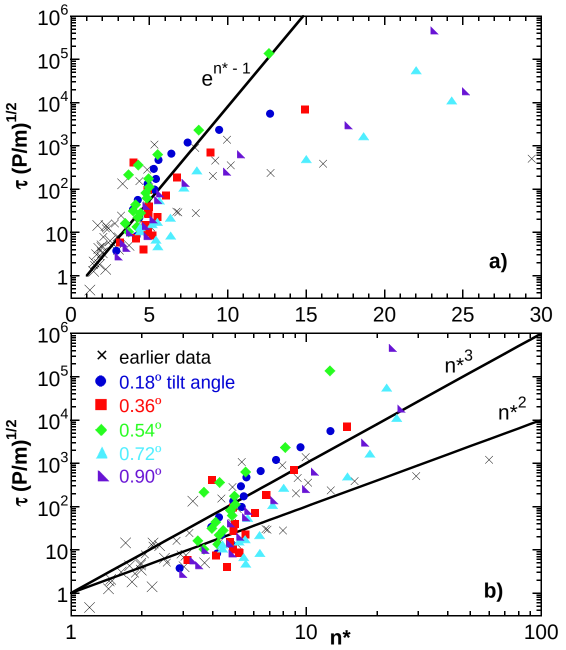


FIG. 5: (nstarvtautilts.pdf) Dimensionless relaxation time, $\tau(P/m)^{1/2}$, where $P$ is pressure and $m$ is small-bead mass, plotted (a) semilogarithmically and (b) logarithmically vs the average number $n^*$ of beads in fast-moving dynamical heterogeneities. The solid symbols are for the system of the main text, with tilt angles as labelled; the $\times$ symbols are for prior data from Refs. [3–5], where $\tau(P/m)^{1/2}$ values are deduced from the known packing fraction according to the scaling plot of the main text. Two power laws and an exponential are shown as guides to the eye; they are forced to go through $(1, 1)$ and are not actual fits.

for $\tau \sim 1/T_{\rm eff}{}^{2.0\pm0.5}$ and $n^* \sim 1/T_{\rm eff}{}^{0.7\pm0.2}$. Altogether the power-law relation for the number $n^*$ of grains in the fast-moving regions as a function of relaxation time $\tau$ may thus be written dimensionlessly as

$$n^* \propto \left[\tau(P/m)^{1/2}\right]^{0.35\pm0.1} \qquad (1)$$

where $P$ is the 2d-pressure (force/length) and $m$ is the small-bead mass. Unfortunately the scatter in the data is large, and it is not feasible to substantially extend the dynamic range in order to obtain better precision on the fitting parameters.


[1] R. P. Ojha, A. R. Abate, and D. J. Durian, Phys. Rev. E **71**, 016313 (2005).
[2] A. R. Abate and D. J. Durian, Phys. Rev. E **74**, 031308 (2006).
[3] A. R. Abate and D. J. Durian, Phys. Rev. E **76**, 021306 (2007).
[4] A. S. Keys, A. R. Abate, S. C. Glotzer, and D. J. Durian, Nature Phys. **3**, 260 (2007).
[5] A. R. Abate and D. J. Durian, Phys. Rev. Lett. **101**, 245701 (2008).
[6] M. Marin, D. Risso, and P. Cordero, J. Comput. Phys. **109**, 306 (1993).
[7] M. Isobe, Int. J. Mod. Phys. C **10**, 1281 (1999).
[8] N. Lačević, F. Starr, T. Schrøder, and S. Glotzer, J. Chem. Phys. **119**, 7372 (2003).
[9] C. Toninelli, M. Wyart, L. Berthier, G. Biroli, and J. P. Bouchaud, Phys. Rev. E **71**, 041505 (2005).
[10] L. Berthier, G. Biroli, J.-P. Bouchaud, L. Cipelletti, and W. van Saarloos, eds., *Dynamical heterogeneities in glasses, colloids, and granular media* (Oxford University Press, 2011).
[11] L. Berthier, Physics **4**, 42 (2011).
[12] H. Katsuragi, A. R. Abate, and D. J. Durian, Soft Matter **6**, 3023 (2010).
[13] K. N. Nordstrom, J. P. Gollub, and D. J. Durian, Phys. Rev. E **84**, 021403 (2011).
